# Supplementary material for: Accelerating Auxiliary-Field Quantum Monte Carlo Simulations of Solids with Graphical Processing Unit
Source: arXiv:2003.09468 ancillary file (2020-03-20)
Supplement: Supplementary file 1 [file supplement.pdf]

# Supplementary information for 'Improving the efficiency of Auxiliary-field quantum Monte Carlo calculations of solids'

Fionn D. Malone, Shuai Zhang, and Miguel A. Morales*

*Lawrence Livermore National Laboratory, Livermore, California 94550, USA*

E-mail: moralessilva2@llnl.gov

## AFQMC Calculations

In this section we detail the convergence of the AFQMC results to the complete basis set (CBS) and thermodynamic limit. All mean field simulations were performed using PySCF[1].

### A Correlation Consistent Basis Set

To construct the modified correlation consistent basis set used in the main text we took the valence states from GTH-TZVP basis sets and the virtuals from the Burkatzki-Filippi-Dolg (BFD) basis set[2]. The basis sets are available with the raw data repositiory at Ref. 3. This choice was motivated by the desire to use the same pseudopotential for all results reported in the work. To test this slightly ad-hoc basis set we carefully examined the convergence of the AFQMC total energies in both the atomic and solid state. In Fig. 3 we first show that the atomic energy extrapolates smoothly with the cardinality of the basis set $X$, where we assumed the usual form of $E_c(X) = E_c(\infty) + aX^{-3}$. In Fig. 2 we show that the AFQMC energies also converge smoothly with the basis set size in solid state simulations. Also plotted

are the AFQMC results using GTH basis sets where no obvious convergence with basis set size is observed. Finally, in Fig. 3 we demonstrate the smooth convergence for different supercell sizes.

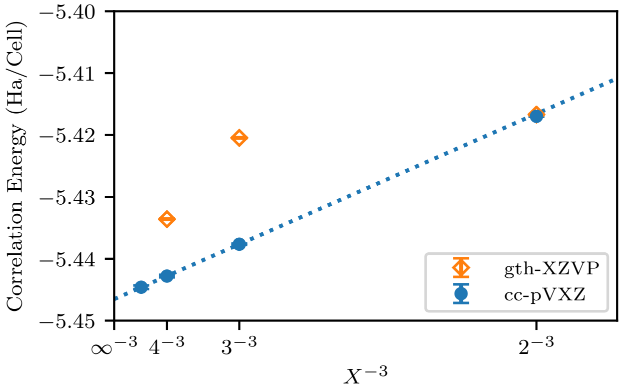


Figure 1: Convergence of AFQMC correlation energy with the cardinality of the basis set $X$ for the triplet ground state of an isolated carbon atom with the gth-pade pseudopotential.

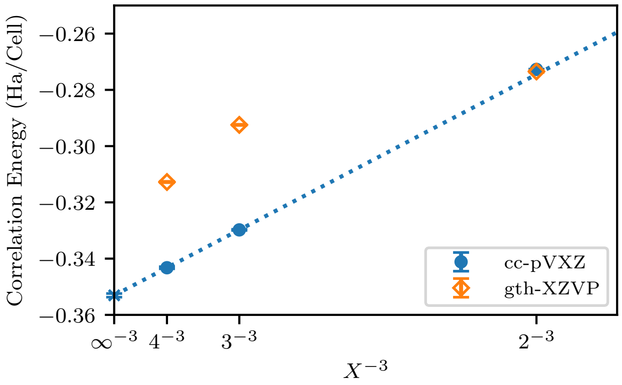


Figure 2: Basis set extrapolation of the AFQMC correlation energy for the $3 \times 3 \times 3$ supercell of Carbon (Diamond) with the cardinality of the basis set $X$. As expected the correlation-consistent basis sets (cc-pVXZ) smoothly extrapolate with a $X^{-3}$ behavior. Also plotted are the AFQMC correlation energies in the gth basis sets (DZVP, TZVP, QZV2P) which do not appear to smoothly extrapolate with basis set size.

## Size Corrections

In Fig. 4 we plot the size correction $\Delta E(N_k) = E(\infty) - E(N_k)$ for the different basis set sizes considered in the text. We see that the basis set dependendence of the size correction

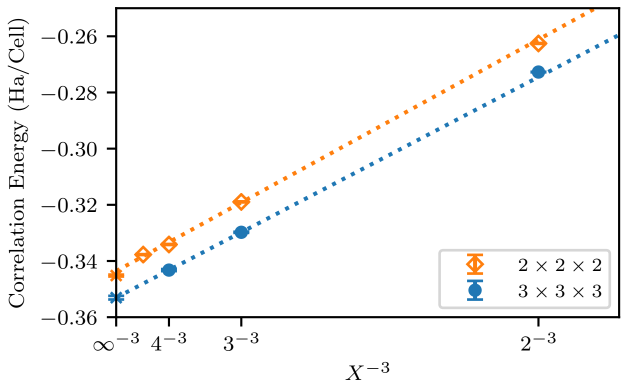


Figure 3: Convergence of AFQMC correlation energy with the cardinality of the basis set $X$ for a $2 \times 2 \times 2$ and $3 \times 3 \times 3$ supercell of Carbon (Diamond).

is weak beyond the $2 \times 2 \times 2$ supercell.

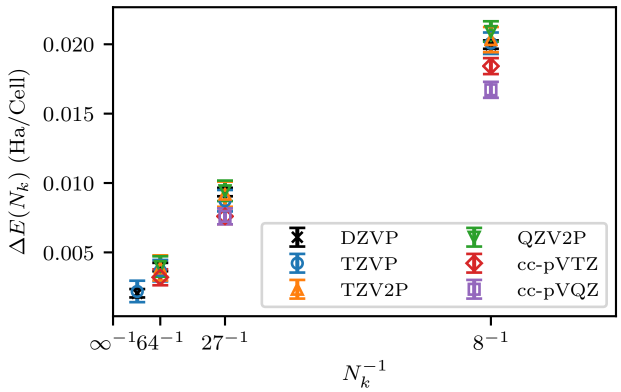


Figure 4: Finite size correction $\Delta E(N_k)$ (see main text for definition) as a function supercell size $(N_k)$ for the basis sets considered in this work.

## Hartree–Fock Energy

For the cohesive energies reported in the main text we separately converged the (restricted) Hartree–Fock energy and correlation energy of the solid state AFQMC calculations. For the GTH basis sets we performed an exponential extrapolation assuming a functional form[4] of $E(N_k) = E(\infty) + a \exp(-bN_k^{1/3})$ for $N_k \in [3, 6]$. In Fig. 5 we plot the convergence of the Hartree–Fock energy to its extrapolated value for the GTH-DZVP and GTH-TZVP basis

sets. The data and extrapolated values are listed in Table 1

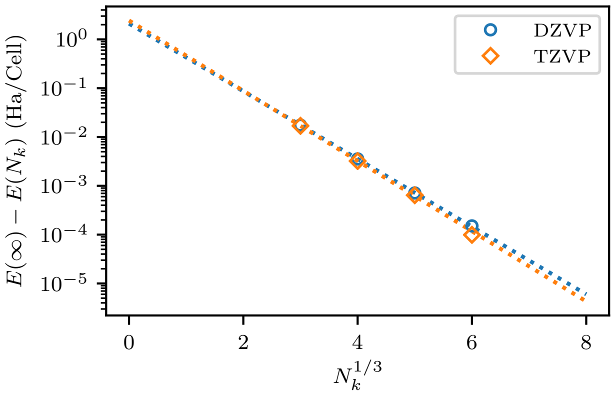


Figure 5: Convergence of Hartree–Fock energy with the total number of $k$-points $N_k$.

Table 1: Hartree–Fock total energies calculated using the truncated Coulomb interaction[5].

| $N_k^{1/3}$ | DZVP | TZVP |
|---|---|---|
| 3 | -11.0742 | -11.0779 |
| 4 | -11.0881 | -11.0916 |
| 5 | -11.0900 | -11.0942 |
| 6 | -11.0915 | -11.0947 |
| $\infty$ | -11.0917 | -11.0948 |

For the correlation consistent basis set we first performed a (D,T,Q) basis set extrapolation[6] the of the Hartree–Fock energy for the $2 \times 2 \times 2$ and $3 \times 3 \times 3$ $k$-point mesh. We then applied a size correction based on the TZVP gth basis set in the same $k$-point mesh $\Delta E_{\mathrm{HF}}(N_k) = E_{\mathrm{HF}}^{\mathrm{TZVP}}(\infty) - E_{\mathrm{HF}}^{\mathrm{TZVP}}(N_k)$. This lead to a consistent value of approximately -11.103 Ha/Cell. A similar value is found if the DZVP Hartree–Fock size correction is used. We estimate this energy is accurate to 1 mHa/Cell. The correlation consistent HF energies are given in Table 2 and Table 3.

# Estimation of Remaining Error

In this section we examine any remaining phaseless error in the AFQMC results by comparing the CCSD, CCSD(T) and selected heat-bath configuration interaction (SHCI) total energies.

Table 2: Hartree–Fock total energies calculated using modified correlation consistent basis sets. Energies are in Ha/Cell. The basis set extrapolated value for a given $k$-point mesh was determined assuming an exponential form[6] using the (D,T,Q) energies.

| $N_k^{1/3}$ | cc-pVDZ | cc-pVTZ | cc-pVQZ | CBS |
|---|---|---|---|---|
| 2 | -11.028529 | -11.039730 | -11.040571 | -11.0406 |
| 3 | -11.040620 | -11.089690 | -11.099099 | -11.1020 |

Table 3: Size corrected correlation consistent Hartree–Fock energies.

| $N_k^{1/3}$ | $E_{\mathrm{HF}}(\mathrm{CBS})$ | $\Delta E_{\mathrm{HF}}^{\mathrm{TZVP}}(N_k)$ | $E_{\mathrm{HF}}(N_k = \infty)$ |
|---|---|---|---|
| 2 | -11.0406 | -0.0611 | -11.1017 |
| 3 | -11.1020 | -0.0013 | -11.1033 |

The SHCI energies were calculated with the DICE code[7,8]. CCSD, CCSD(T) and MP2 energies were calculated using PySCF[1]. In Fig. 6 we plot the error in the various methods relative to converged (exact) SHCI total energies in the unit cell of Carbon (Diamond). We can see that the phaseless error amounts to approximately 6 mHa/Cell. In comparison the CCSD makes an error of approximately 14 mHa/Cell, which grows slightly with the basis set size. CCSD(T) shows essentially no dependence on basis set size and makes a maximum error of 3 mHa/Cell.

In Fig. 7 we plot the AFQMC error in the atomic energy as a function of basis set size. We see that it has a weak dependence on basis set size and is approximately 6 mHa. We can see that the error between the atom and solid calculation approximately cancel which may explain the excellent agreement for the cohesive energy reported in the main text. This is assuming the phaseless error does not grow significanlty with system size (on a per atom basis).

# AFQMC Data

We list in Tables 4 to 6 the AFQMC total energies used to make the figures in the main text. Note that for the atomic calculations we used a timestep of 0.005 $\mathrm{Ha}^{-1}$. For the solid state calculations we found that time step extrapolation was necessary to ensure a smooth

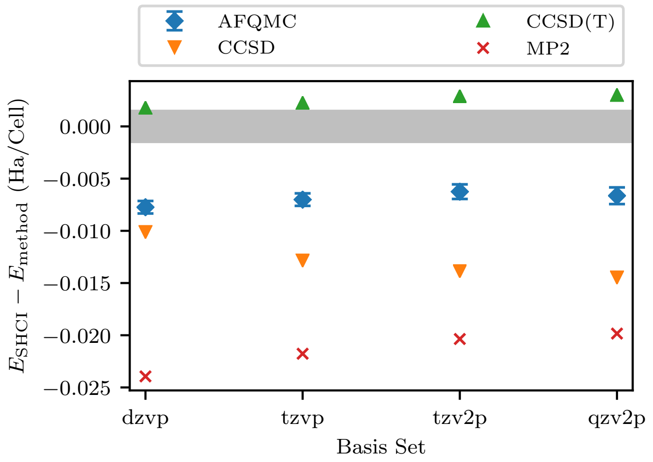


Figure 6: Error in single determinant AFQMC compared to exact HCI results for the primitive cell of carbon. Also plotted are the errors in CCSD, CCSD(T) and MP2 theory also measured relative to HCI. The shaded grey region represents chemical accuracy ±1.6 mHa/Cell. The MP2 energies have been shifted by -0.18 Ha/Cell to be visible on the figure.

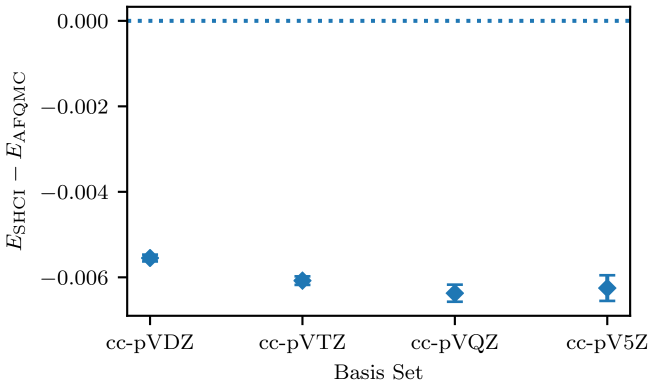


Figure 7: Comparison between (single determinant) AFQMC and SHCI total energies for the isolated carbon atom in the correlation consistent basis sets constructed in this work .

extrapolation to the thermodynamic limit. This was particularly found to be the case beyond $N_k = 64$. The results in Table 4 are thus all time step extrapolated using a two-point linear extrapolation from $\Delta\tau = (0.01, 0.005)$ $\text{Ha}^{-1}$.

Table 4: Raw AFQMC energies and Hartree–Fock energies for system sizes and basis sets considered in this work. Energies are in Ha/Cell.

| Basis | $N_k^{1/3}$ | Energy | $E_{\text{HF}}$ | $E_{\text{cor}}$ |
|---|---|---|---|---|
| DZVP | 2 | -11.2914(4) | -11.028529 | -0.2628(4) |
| | 3 | -11.3632(3) | -11.089696 | -0.2735(3) |
| | 4 | -11.3742(1) | -11.095312 | -0.2789(1) |
| | 5 | -11.3756(2) | -11.094831 | -0.2808(2) |
| TZVP | 2 | -11.3148(4) | -11.033744 | -0.2811(4) |
| | 3 | -11.3859(2) | -11.093408 | -0.2924(2) |
| | 4 | -11.3963(5) | -11.098809 | -0.2975(5) |
| | 5 | -11.3970(4) | -11.098051 | -0.2990(4) |
| TZV2P | 2 | -11.3336(3) | -11.037046 | -0.2965(3) |
| | 3 | -11.4045(3) | -11.096849 | -0.3077(3) |
| | 4 | -11.4152(8) | -11.102207 | -0.3130(8) |
| QZV2P | 2 | -11.3394(3) | -11.038099 | -0.3013(3) |
| | 3 | -11.4102(2) | -11.097416 | -0.3128(2) |
| | 4 | -11.4209(4) | -11.102694 | -0.3182(4) |
| cc-pVTZ | 2 | -11.3587(2) | -11.039730 | -0.3190(2) |
| | 3 | -11.4289(2) | -11.099099 | -0.3298(2) |
| cc-pVQZ | 2 | -11.3747(2) | -11.040571 | -0.3341(2) |
| | 3 | -11.4432(4) | -11.099933 | -0.3432(4) |
| cc-pV5Z | 2 | -11.3783(2) | -11.040620 | -0.3377(2) |

Table 5: Size extrapolated AFQMC correlation energies for the basis sets considered. The error bar gives an estimate for the error in the extrapolation. Energies are in Ha atomic units. *The cc-pVQZ data contains a size correction from the cc-pVTZ data.

| basis | $E_{\text{cor}}$ |
|---|---|
| DZVP | -0.2828(3) |
| TZVP | -0.3012(8) |
| TZV2P | -0.317(1) |
| QZV2P | -0.3222(7) |
| cc-pVTZ | -0.337(1) |
| cc-pVQZ* | -0.351(1) |

Table 6: AFQMC total energies for the triplet ground state of a Carbon atom. For the GTH basis sets the counterpoise corrected (CP) energies are also listed. The counterpoise corrected energies were computed by surrounding a carbon atom at the origin by a 'shell' of ghost atoms in the diamond crystal structure. The PySCF simulation was then performed by setting 'cell.dimension = 0' with the gth basis sets and pseudopotential. We used Gaussian density fitting for the integrals and the subsequent AFQMC simulation. Energies are in Hartree atomic units.

| basis | Energy | Energy (CP) |
|---|---|---|
| dzvp | -5.41669(8) | -5.41826(9) |
| tzvp | -5.4205(1) | -5.42279(9) |
| tzv2p | -5.4270(1) | -5.4289(1) |
| qzv2p | -5.4336(1) | -5.4343(1) |
| cc-pvdz | -5.41698(8) | - |
| cc-pvtz | -5.4376(1) | - |
| cc-pvqz | -5.4428(2) | - |
| cc-pv5z | -5.4446(3) | - |
| CBS | -5.4465(3) | - |

## References

(1) Sun, Q.; Berkelbach, T. C.; Blunt, N. S.; Booth, G. H.; Guo, S.; Li, Z.; Liu, J.; McClain, J. D.; Sayfutyarova, E. R.; Sharma, S.; Wouters, S.; Chan, G. K. L. PySCF: the Python-based simulations of chemistry framework. *WIREs Comput. Mol. Sci.* **2017**, *8*, e1340.

(2) Burkatzki, M.; Filippi, C.; Dolg, M. Energy-consistent pseudopotentials for quantum Monte Carlo calculations. *J. Chem. Phys.* **2007**, *126*, 234105.

(3) All simulation data is available at [url to be inserted].

(4) McClain, J.; Sun, Q.; Chan, G. K.-L.; Berkelbach, T. C. Gaussian-based coupled-cluster theory for the ground-state and band structure of solids. *J. Chem. Theory Comput.* **2017**, *13*, 1209–1218.

(5) Spencer, J.; Alavi, A. Efficient calculation of the exact exchange energy in periodic systems using a truncated Coulomb potential. *Phys. Rev. B* **2008**, *77*, 193110.

(6) Helgaker, T.; Klopper, W.; Koch, H.; Noga, J. Basis-set convergence of correlated calculations on water. *J. Chem. Phys.* **1997**, *106*, 9639–9646.

(7) Sharma, S.; Holmes, A. A.; Jeanmairet, G.; Alavi, A.; Umrigar, C. J. Semistochastic Heat-Bath Configuration Interaction Method: Selected Configuration Interaction with Semistochastic Perturbation Theory. *J. Chem. Theory Comput.* **2017**, *13*, 1595–1604.

(8) Holmes, A. A.; Tubman, N. M.; Umrigar, C. J. Heat-Bath Configuration Interaction: An Efficient Selected Configuration Interaction Algorithm Inspired by Heat-Bath Sampling. *J. Chem. Theory Comput.* **2016**, *12*, 3674–3680.
